# Supplementary material for: Topological insulators on fractal lattices: A general principle of construction
Source: arXiv:2407.13767 ancillary file (2024-12-26)
Supplement: Supplementary file 1 [file Supplementary_Fractal3Methods_TIs.pdf]

# Supplemental Material:
# Topological insulators on fractal lattices: A general principle of construction

Daniel J. Salib,[1] Aiden J. Mains,[1] and Bitan Roy[1]

[1] *Department of Physics, Lehigh University, Bethlehem, Pennsylvania, 18015, USA*

(Dated: December 5, 2024)

Supplemental Material contains (a) phase diagrams in the $(M, \tilde{B})$ plane for Sierpiński carpet fractal lattices, derived using all three methods [see Sec. S1 and Fig. S1] and (b) stability of all the topological insulators (TIs) in disordered fractal lattices [see Sec. S2, Fig. S2 and Table I].

## S1. PHASE DIAGRAM IN THE $(M, \tilde{B})$ PLANE

In this section, we discuss the phase diagram of the generalized Qi-Wu-Zhang model on the Sierpiński carpet fractal lattices, obtained by employing three methods (Method 1, 2, and 3), which we discuss in detail in the main manuscript. The results are shown in Fig. S1. In Fig. S1(a) and (b), we show the phase diagrams in the $(M, \tilde{B})$ plane, obtained from both Method 1 and Method 2, which yield identical results. Fig. S1(a) and (b) refer to Sierpinski carpet fractal lattices of third and fourth generation, respectively. In Fig. S1(c), we show the same phase diagram, obtained from Method 3 on a third generation Sierpiński carpet fractal lattice. We now discuss some of their salient features.

By comparing the phase diagrams in Fig. S1(a) and (b), we note the following features. The parameter regimes on the $(M, \tilde{B})$ plane over which the topological insulators with Bott index (BI) equal to 1 and $-2$ are realized remain *almost* the same (within numerical accuracy) for the Sierpiński carpet fractal lattices of third and fourth generations, assuring their ultimate stability in the thermodynamic limit. On the other hand, the region in the $(M, \tilde{B})$ plane over which a topological insulator with BI $= -1$ is realized changes mildly for any finite $\tilde{B}$. However, the range of $M$ over which this phase is realized when $\tilde{B} = 0$, remains the same for third and fourth generation Sierpiński carpet fractal lattices, assuring the ultimate stability of this phase in the thermodynamic limit on the $\tilde{B} = 0$ axis. Thus, topological insulators with BI $= \pm 1$ and 2 can be realized on Sierpiński carpet fractal lattice within certain parameter regimes in the thermodynamic limit. We also note the appearance of small patches of a BI $= 1$ phase in Fig. S1(b) for fourth generation Sierpiński carpet fractal lattice, which is absent on its third generation cousin. We thus cannot assert any stability of such a phase in the thermodynamic limit.

Finally, we examine the phase diagram from Fig. S1(c), obtained using Method 3, on a third generation Sierpiński carpet fractal lattice. This phase diagram is identical to the one for a parent square lattice of $L = 27$, which is also

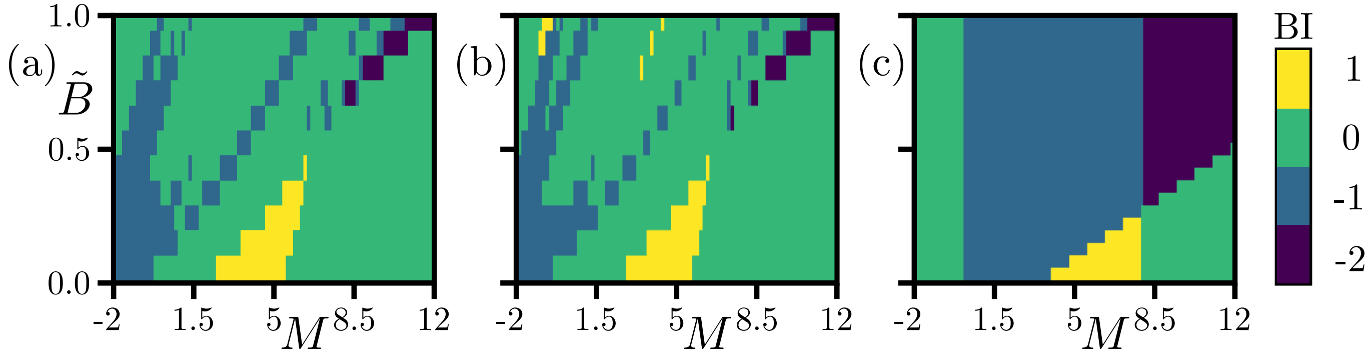


Figure S1. Phase diagrams of Sierpiński carpet fractal lattices of (a) third generation and (b) fourth generation, obtained from Method 1 and Method 2, yielding identical results, and (c) third generation, obtained from Method 3, yielding identical results as in the parent square lattice of $L = 27$. See Sec. S1 for details. Here, we set $t_1 = t_2 = 1$, but along the $\tilde{B} = 0$ line we also set $t_2 = 0$ to switch of any hopping along the diagonal directions in the parent square lattice Hamiltonian.

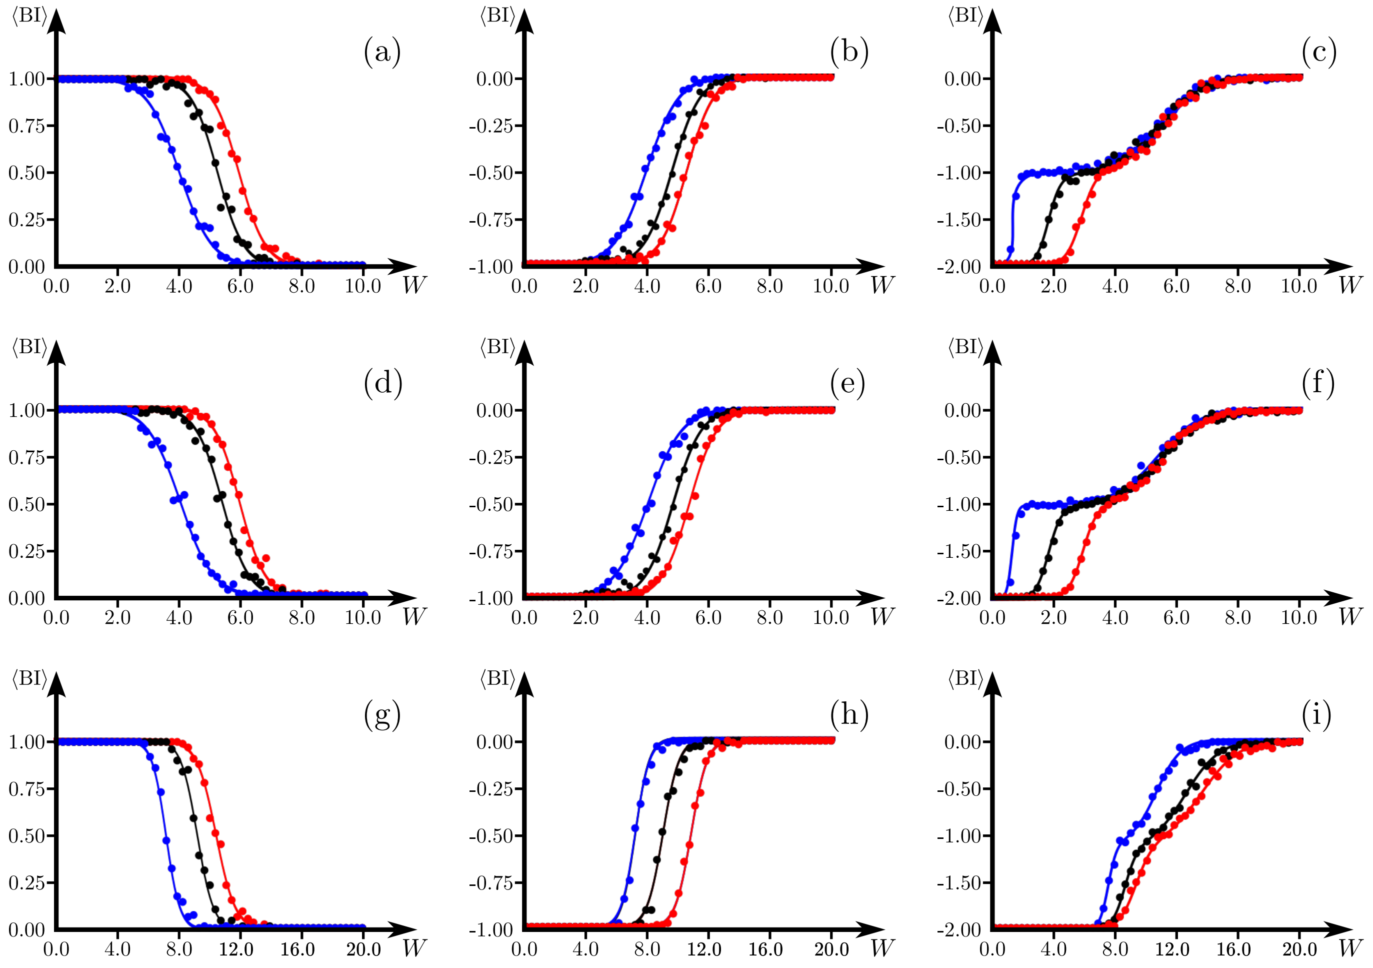

Figure S2. Disorder-averaged Bott index ⟨BI⟩, obtained after averaging over 100 independent and random disorder realizations, as a function of the disorder strength ($W$) for various topological insulators with the Bott index BI $= \pm 1$ and 2 in the clean limit on a third generation Sierpiński carpet fractal lattice. The calculation is performed with the real space Hamiltonian constructed from Method 1 [(a)-(c)], Method 2 [(d)-(f)], and Method 3 [(g)-(i)]. The parameter values are tabulated in Table I. In all the cases, topological insulators with quantized ⟨BI⟩ remain stable in the weak disorder regime, while normal or trivial insulators with ⟨BI⟩ $= 0$ appear in the strong disorder regime. See Sec. S2 for details.

identical to the one shown in Fig. 1(c) of the main manuscript in terms of either the first Chern number or the Bott index. Therefore, stability of all the topological insulators on Sierpiński carpet fractal lattices can be guaranteed in the thermodynamic limit when we employ Method 3 to compute the corresponding real space Hamiltonian.

## S2. STABILITY OF TOPOLOGICAL INSULATORS ON DISORDERED FRACTAL LATTICES

In this section, we scrutinize the stability of all the topological phases with BI $= \pm 1$ and 2 on a clean Sierpiński carpet fractal lattice in the presence of weak disorder. For concreteness, we consider the effects of random pointlike charge impurities, the dominant source of elastic scattering in any real material. The effect of pointlike random charge impurities is captured by the Hamiltonian

$$H_{\text{dis}} = \sum_{\boldsymbol{r}_i} V(\boldsymbol{r}_i)\tau_0, \tag{S1}$$

where $i$ is the site index, located at $\boldsymbol{r}_i$ and $\tau_0$ is two-dimensional identity matrix. $V(\boldsymbol{r}_i)$ is distributed uniformly and independently within the range $[-W/2, W/2]$, where $W$ denotes the strength of disorder. For each realization of

| **Sub Figure** | **Curve color** | $(t_1, t_2, B, M, \tilde{B})$ | $G$ | $W_c$ | ⟨BI⟩ |
|---|---|---|---|---|---|
| (a) | Red | (1.0, 0.0, 1.0, 6.5, 0.0) | 0.136 | 4.80 | +1 |
| | Black | (1.0, 0.0, 1.0, 6.0, 0.0) | 0.112 | 3.90 | +1 |
| | Blue | (1.0, 0.0, 1.0, 5.5, 0.0) | 0.066 | 1.98 | +1 |
| (b) | Red | (1.0, 0.0, 1.0, 2.0, 0.0) | 0.140 | 4.64 | -1 |
| | Black | (1.0, 0.0, 1.0, 2.25, 0.0) | 0.118 | 1.96 | -1 |
| | Blue | (1.0, 0.0, 1.0, 2.5, 0.0) | 0.081 | 1.76 | -1 |
| (c) | Red | (1.0, 1.0, 1.0, 10.0, 0.85) | 0.116 | 1.77 | -2 |
| | Black | (1.0, 1.0, 1.0, 10.0, 0.925) | 0.068 | 1.06 | -2 |
| | Blue | (1.0, 1.0, 1.0, 10.0, 0.95) | 0.044 | 0.35 | -2 |
| (d) | Red | (1.0, 0.0, 1.0, 6.5, 0.0) | 0.136 | 3.20 | +1 |
| | Black | (1.0, 0.0, 1.0, 6.0, 0.0) | 0.112 | 2.50 | +1 |
| | Blue | (1.0, 0.0, 1.0, 5.5, 0.0) | 0.066 | 2.00 | +1 |
| (e) | Red | (1.0, 0.0, 1.0, 2.0, 0.0) | 0.140 | 4.10 | -1 |
| | Black | (1.0, 0.0, 1.0, 2.25, 0.0) | 0.118 | 2.33 | -1 |
| | Blue | (1.0, 0.0, 1.0, 2.5, 0.0) | 0.081 | 1.43 | -1 |
| (f) | Red | (1.0, 1.0, 1.0, 10.0, 0.85) | 0.116 | 1.42 | -2 |
| | Black | (1.0, 1.0, 1.0, 10.0, 0.925) | 0.068 | 1.06 | -2 |
| | Blue | (1.0, 1.0, 1.0, 10.0, 0.95) | 0.044 | 0.35 | -2 |
| (g) | Red | (1.0, 0.0, 1.0, 6.0, 0.0) | 2.330 | 8.22 | +1 |
| | Black | (1.0, 0.0, 1.0, 5.0, 0.0) | 1.793 | 6.80 | +1 |
| | Blue | (1.0, 0.0, 1.0, 4.5, 0.0) | 1.223 | 5.36 | +1 |
| (h) | Red | (1.0, 0.0, 1.0, 1.0, 0.0) | 1.907 | 7.83 | -1 |
| | Black | (1.0, 0.0, 1.0, 3.0, 0.0) | 1.804 | 6.06 | -1 |
| | Blue | (1.0, 0.0, 1.0, 3.5, 0.0) | 1.176 | 5.38 | -1 |
| (i) | Red | (1.0, 1.0, 1.0, 10.0, 1.0) | 2.226 | 6.43 | -2 |
| | Black | (1.0, 1.0, 1.0, 10.0, 0.9) | 1.968 | 6.00 | -2 |
| | Blue | (1.0, 1.0, 1.0, 10.0, 0.8) | 1.045 | 5.00 | -2 |

Table I. Parameter values $(t_1, t_2, B, M, \tilde{B})$ (third column) for various subfigures [(a)-(i) in first column] and various curves (color coded, mentioned in the second column) of Fig. S2. In the fourth column, we specify the gap ($G$) between two closest to zero-energy modes, with opposite signs, in clean Sierpiński carpet fractal lattice of third generation. In the fifth column we quote the critical value of disorder $W_c$ up to which the disorder averaged Bott index ⟨BI⟩ retains its various quantized values, mentioned in the sixth column, on both third and fourth generation Sierpiński carpet fractal lattices. The value of $G$, $W_c$, and ⟨BI⟩ are obtained in systems with periodic boundary conditions in both $x$ and $y$ directions.

potential disorder $\mathrm{Tr}[V(\boldsymbol{r_i})] = \Delta \neq 0$. Thus, it is not particle-hole symmetric. However, the particle-hole symmetry is recovered after averaging over a sufficiently large number of independent disorder realizations. To circumvent this issue, we define a quantity $\delta = \Delta/N$, where $N$ is the total number of sites in the system, and subtract $\delta$ uniformly from all the sites. Naturally, $\delta \ll W$, and error introduced in this process is negligible. We perform the numerical simulations with a modified disorder Hamiltonian

$$H_{\rm dis}^{\rm mod} = H_{\rm dis} - \sum_{\boldsymbol{r}_i} \delta \, \tau_0. \tag{S2}$$

Notice that $H_{\rm dis}^{\rm mod}$ preserves the particle-hole symmetry for each disorder realization. Still, each data point is obtained after averaging over 100 independent disorder realizations in systems with periodic boundary conditions in both directions. The results are shown in Fig. S2, which we discuss next.

The results shown in Fig. S2 are obtained from a Sierpiński carpet fractal lattice of third generation. With the real space Hamiltonian, obtained from all the methods, we first identify the parameter values, quoted in Table I, for which the system supports topological insulators with BI = ±1 and 2. We then increase the strength of disorder ($W$) and for each value of $W$ compute the disorder averaged Bott index ⟨BI⟩. From ⟨BI⟩ we identify the critical disorder strength $W_c$ up to which it retains the quantized values. Beyond $W_c$, ⟨BI⟩ deviates from its quantized values and

for sufficiently strong disorder $\langle \mathrm{BI} \rangle = 0$, indicating onset of a trivial or normal insulator. In order to establish the ultimate stability of the topological insulators in the presence of disorder in the thermodynamic limit, we compute $\langle \mathrm{BI} \rangle$ for $W = W_c$ on fourth generation Sierpiński carpet fractal lattices, and find that $\langle \mathrm{BI} \rangle$ retains its quantized value in such systems. These results are qualitatively similar for all three methods of constructing the real space Hamiltonian on the fractal lattice.

We also made the following observation regarding the strength of $W_c$ and the spectral gap $(G)$ between two closest to zero-energy modes of opposite signs, computed in clean systems, for same set of parameter values. The values of $G$ are quoted in the fourth column of Table I. It shows that with increasing $G$, $W_c$ increases monotonically. Therefore, it takes stronger strength of disorder $(W_c)$ to destroy a topological insulator with larger spectral gap $(G)$, which is somewhat expected, as the transition from a topological to trivial insulator takes place via a band gap closing due to increasing disorder in the system.
